# Supplementary material for: As-Plausible-As-Possible: Plausibility-Aware Mesh Deformation Using 2D Diffusion Priors
Source: arXiv:2311.16739 source file (2024-03-30)
Supplement: Supplementary file 1 [file image_list.tex]

\Image{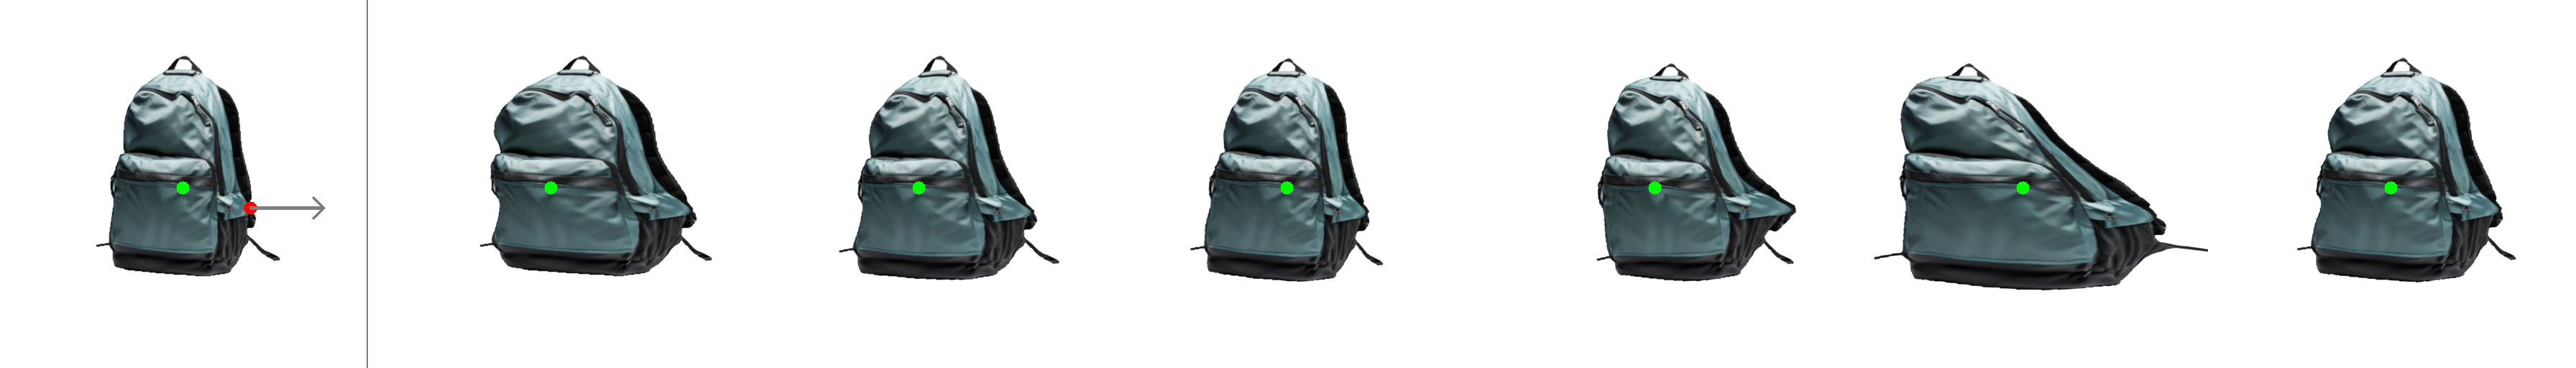} 
\Image{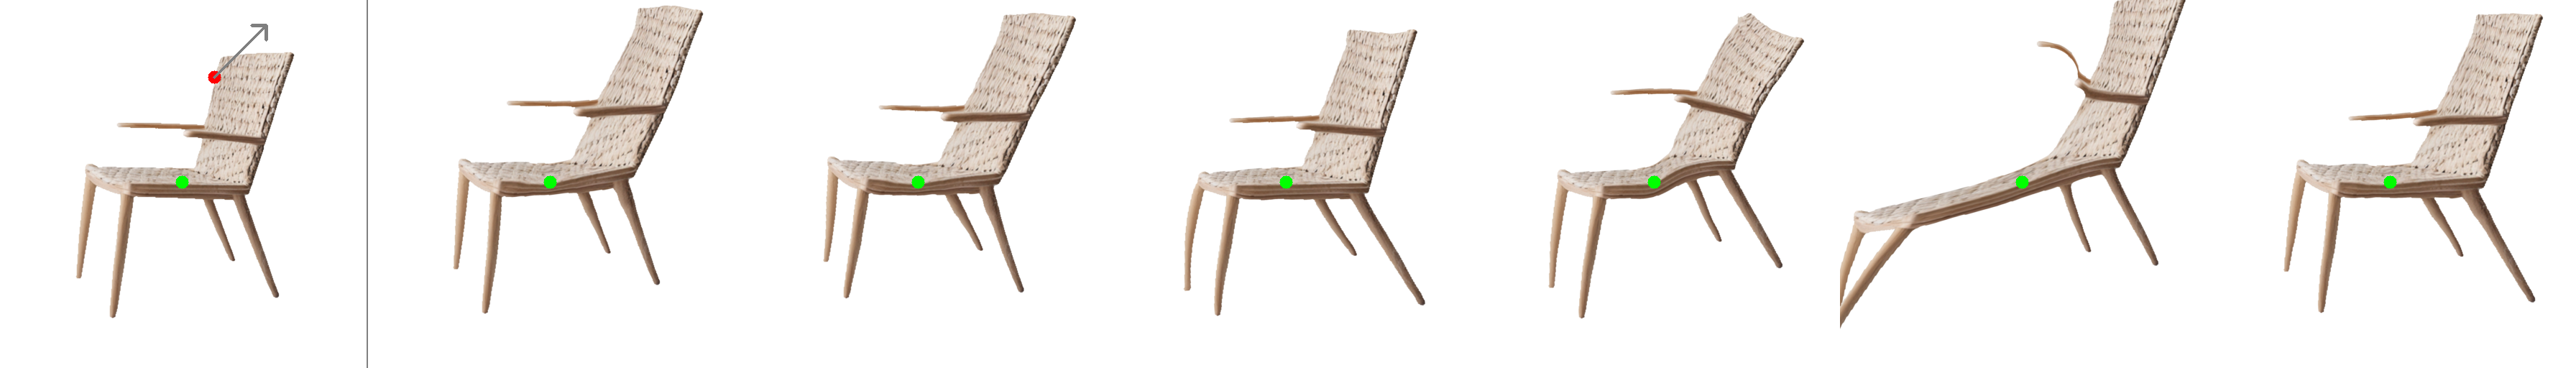} 
\Image{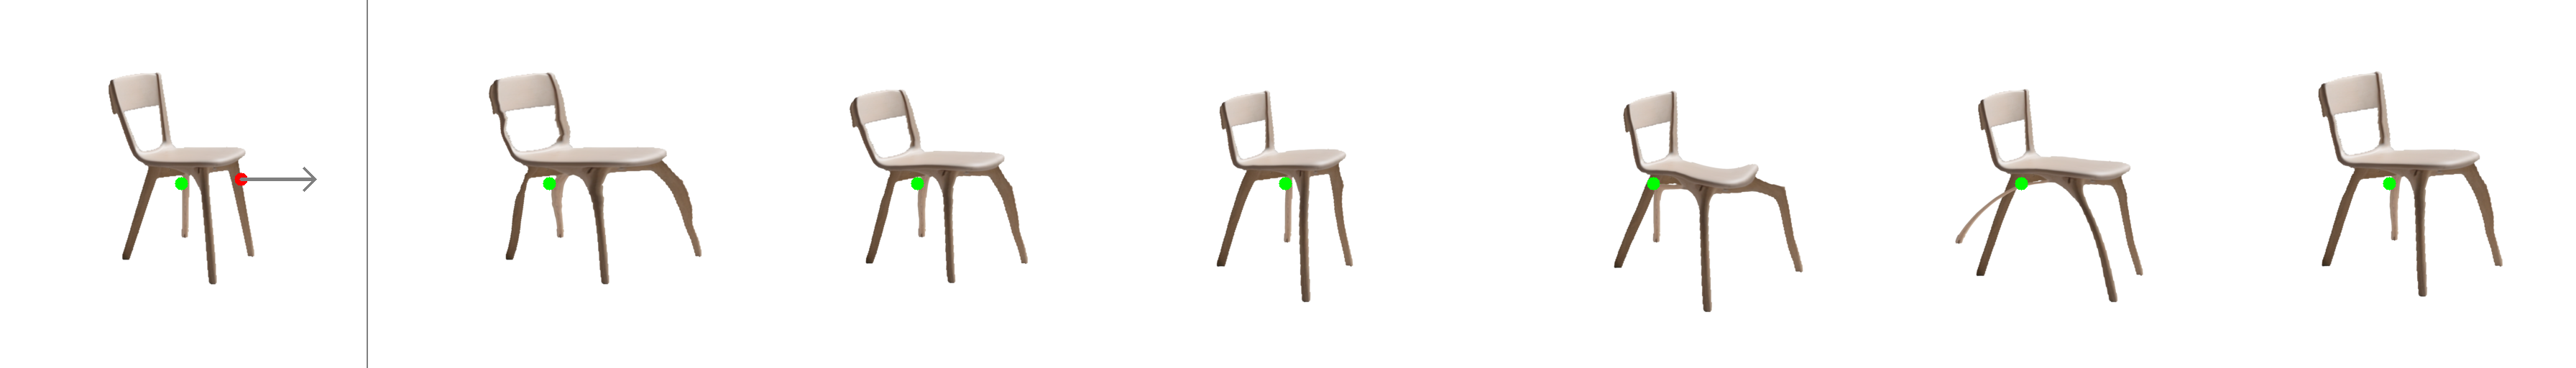} 
\Image{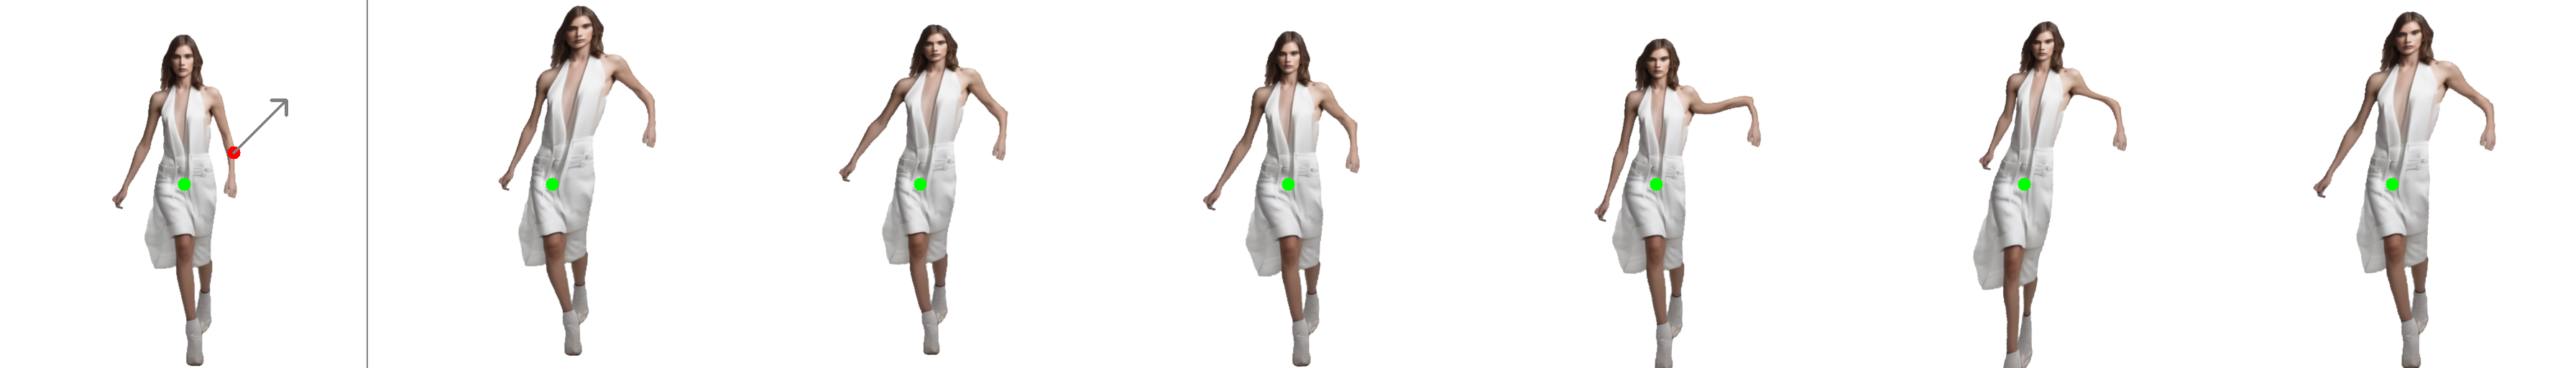} 
\Image{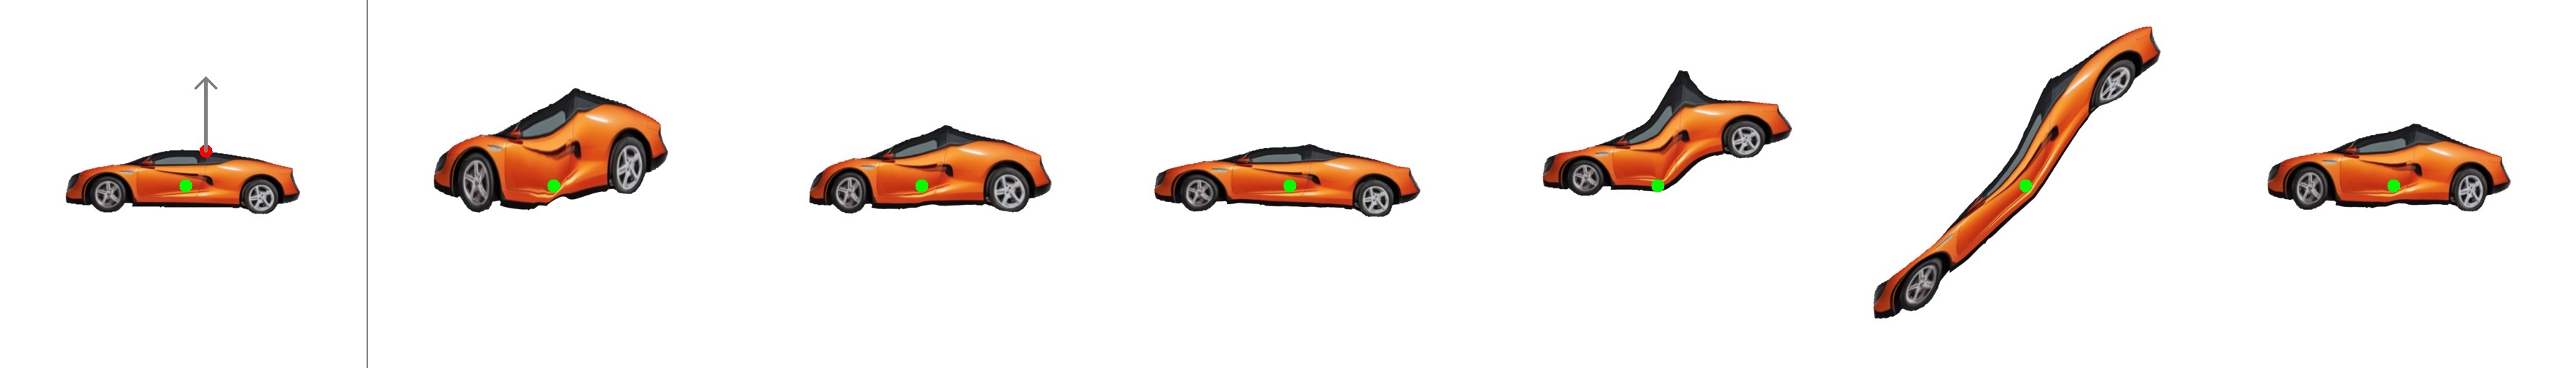} 
\Image{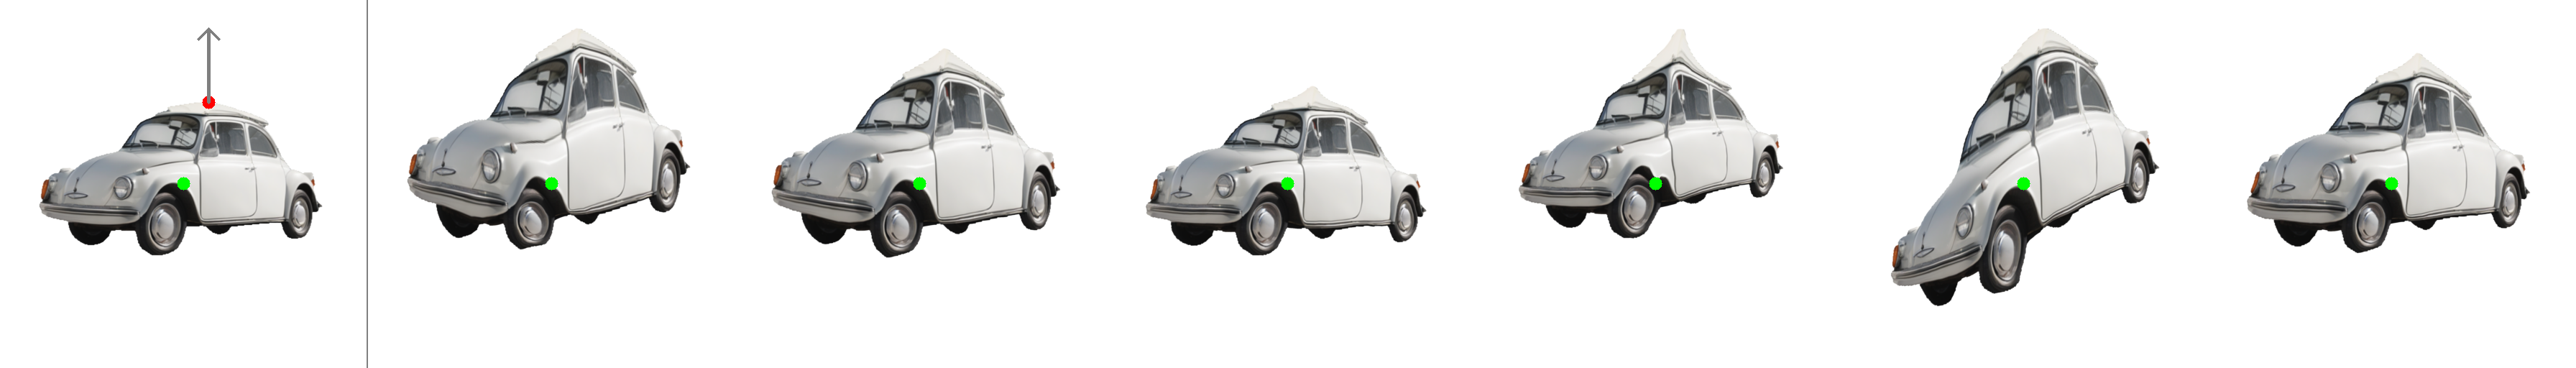} 
\Image{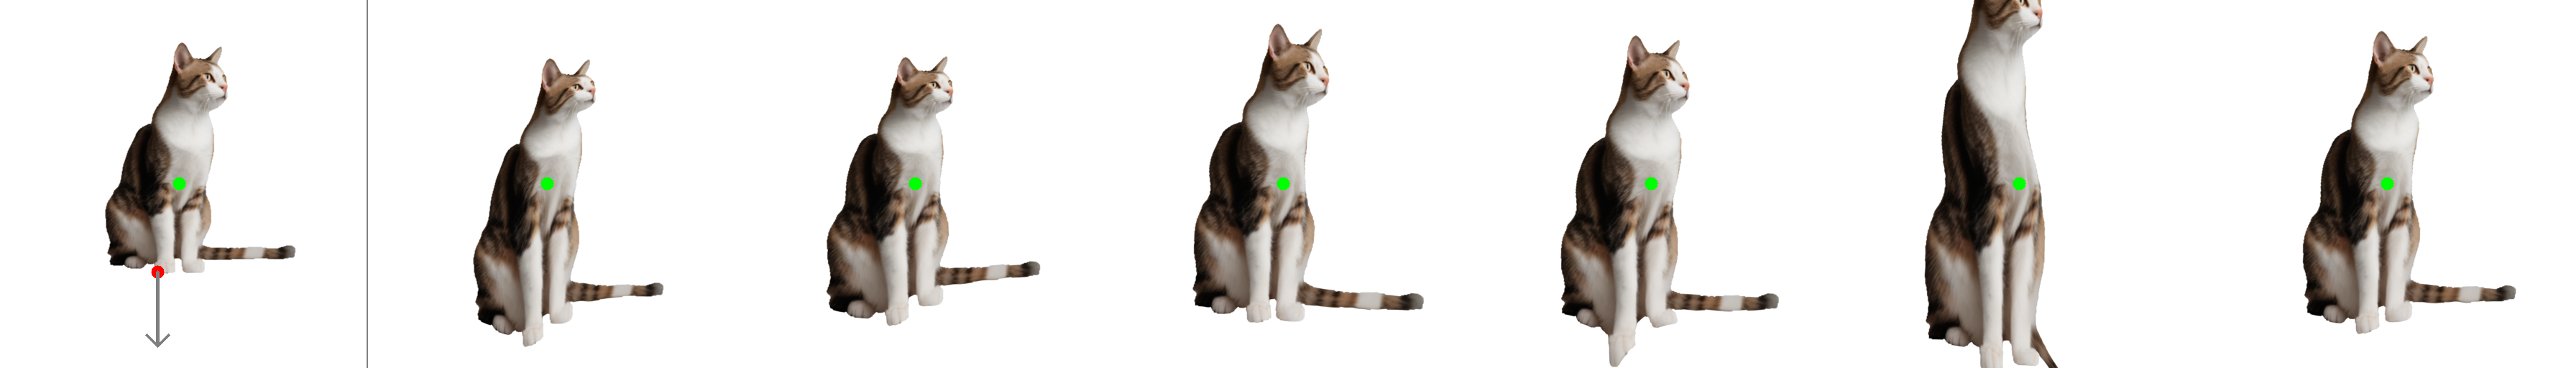} 
\Image{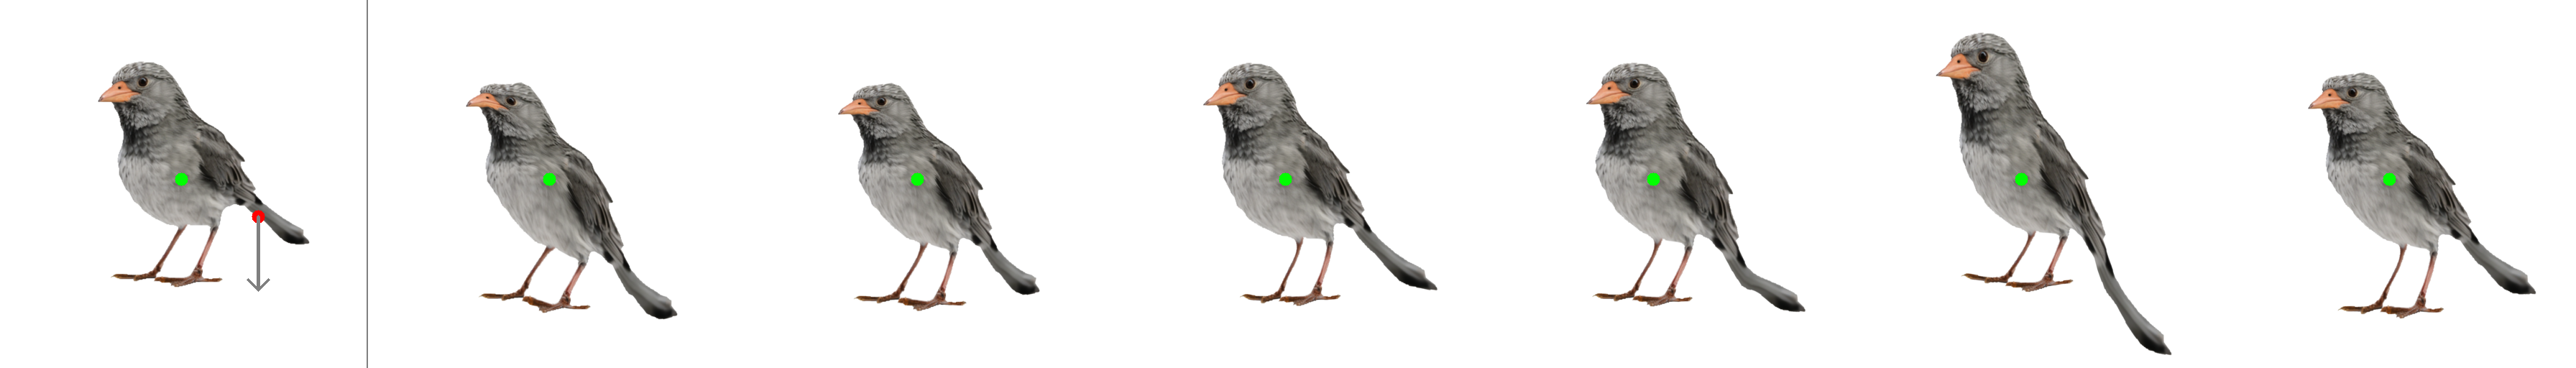} 
\Image{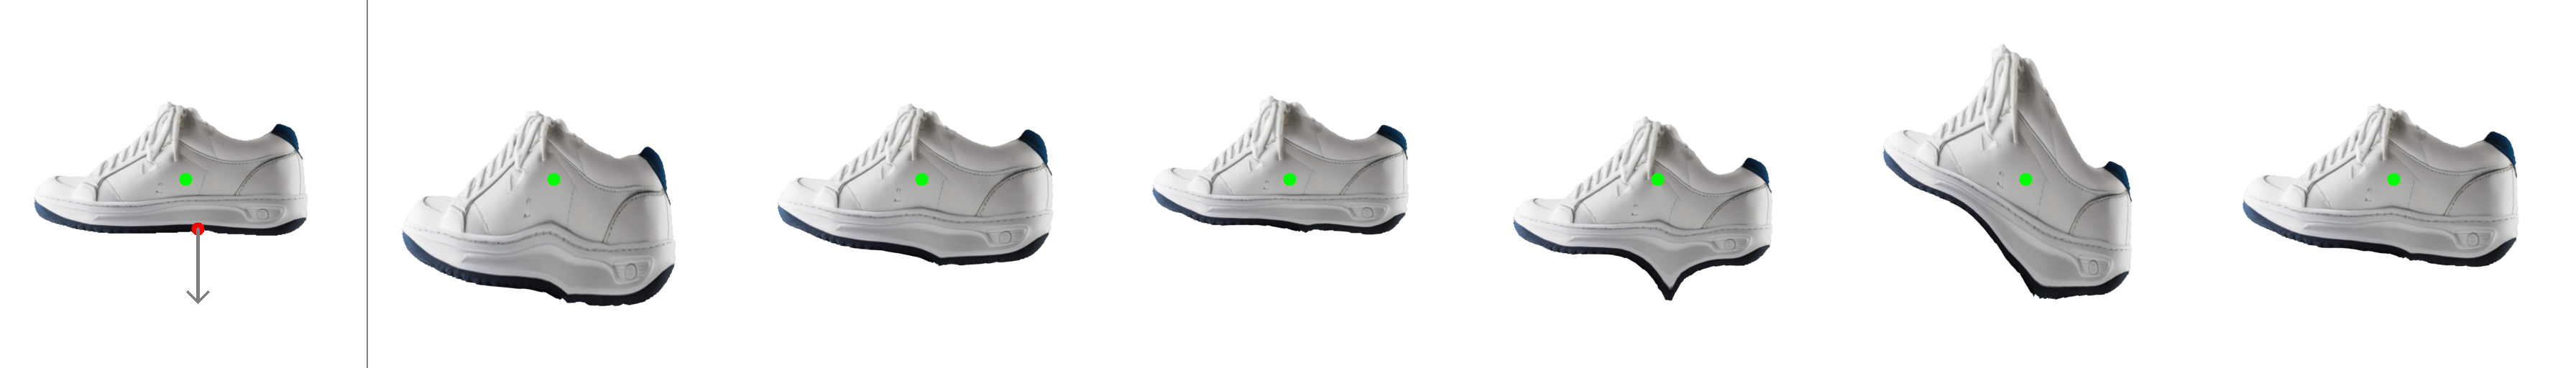} 
\Image{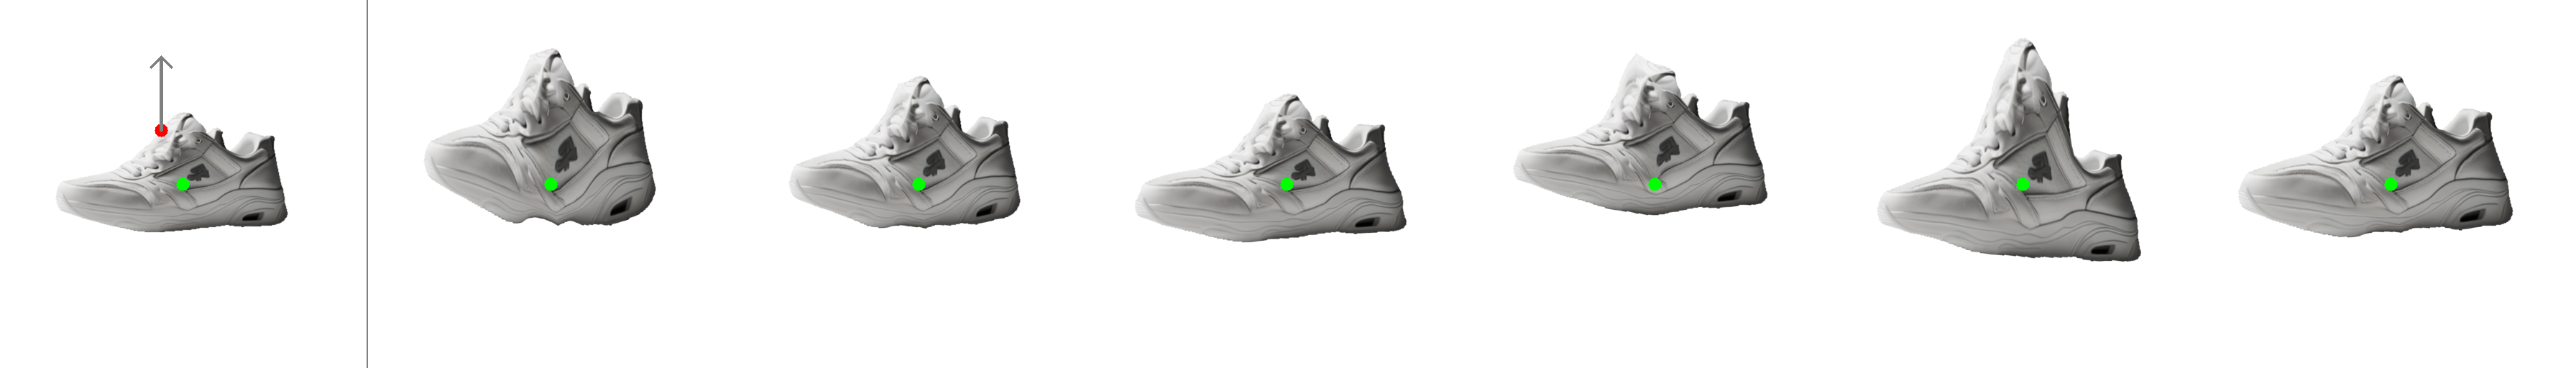} 
\Image{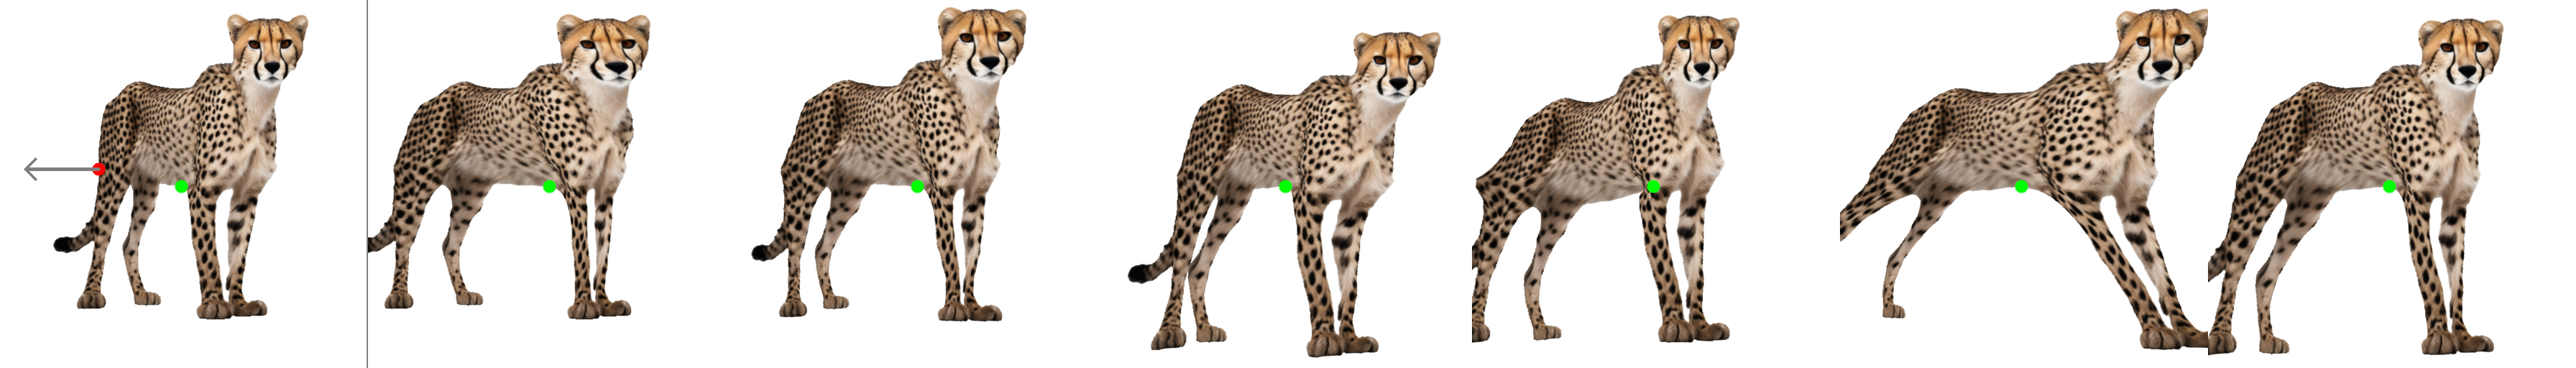} 
\Image{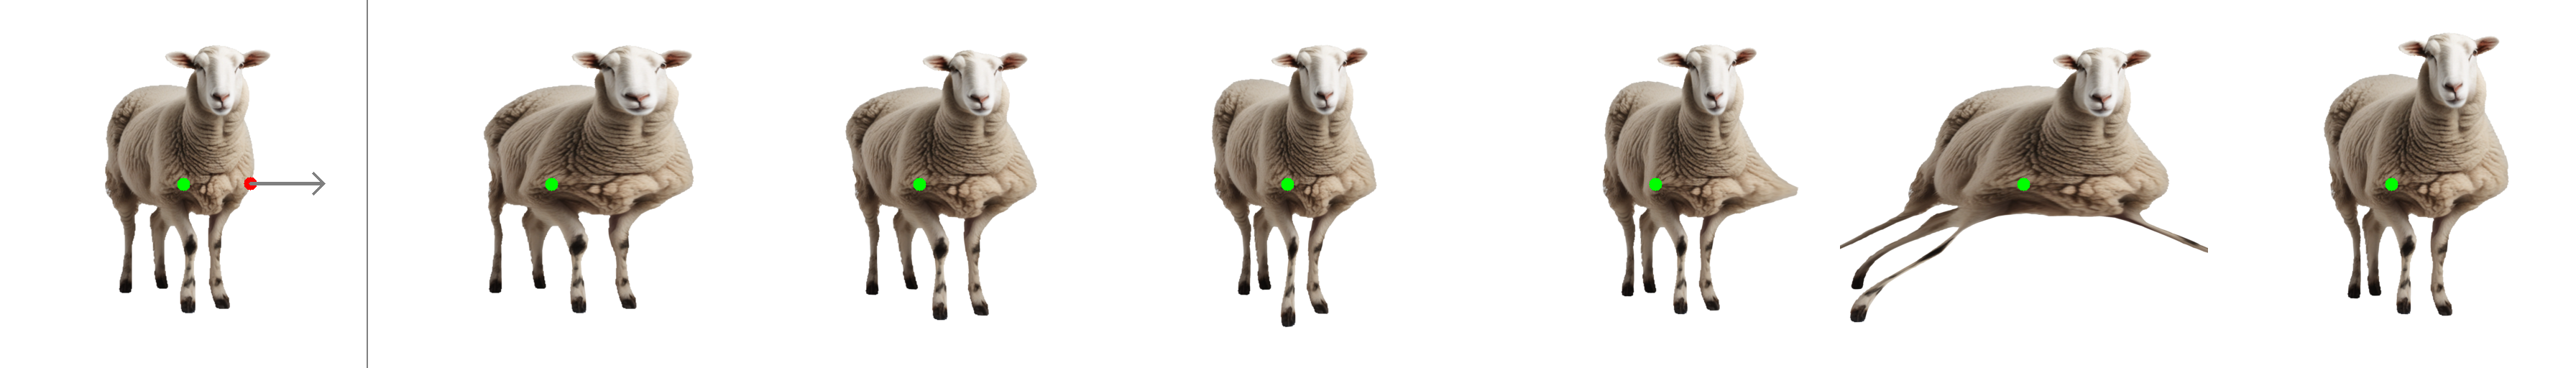} 
\Image{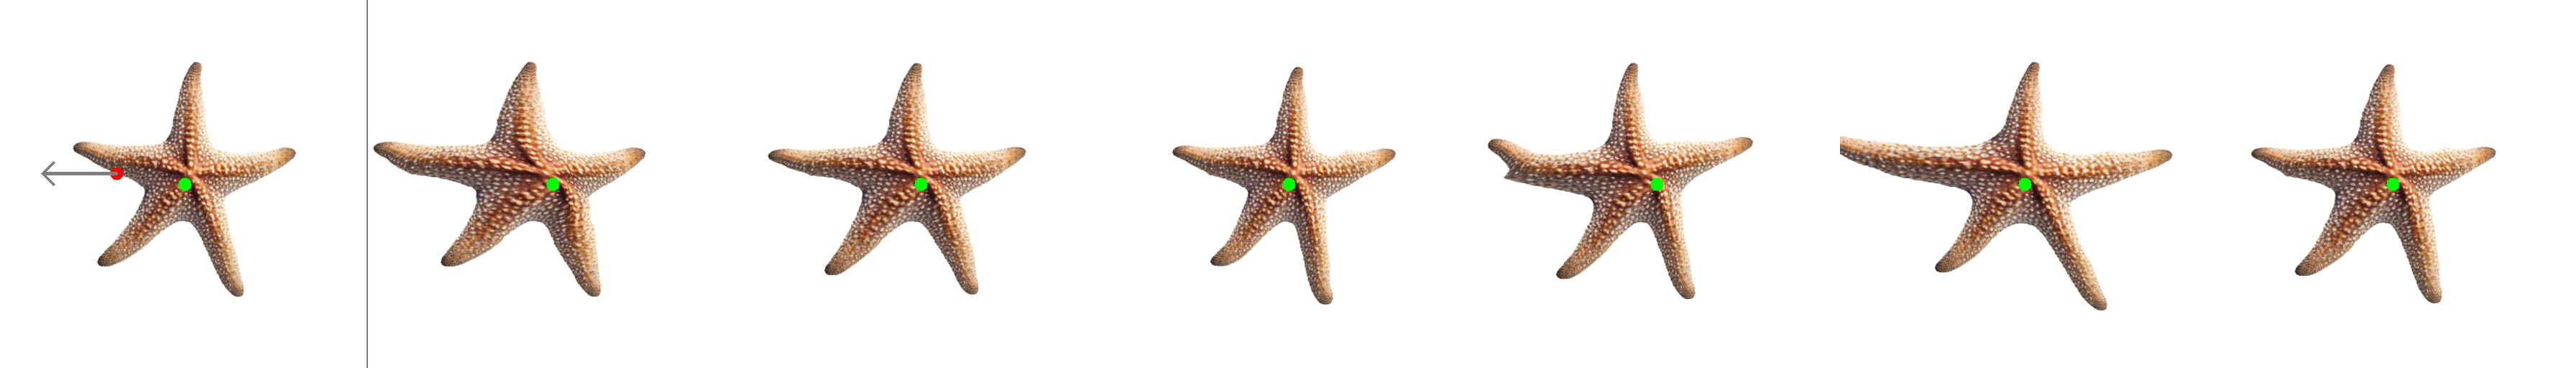} 
\Image{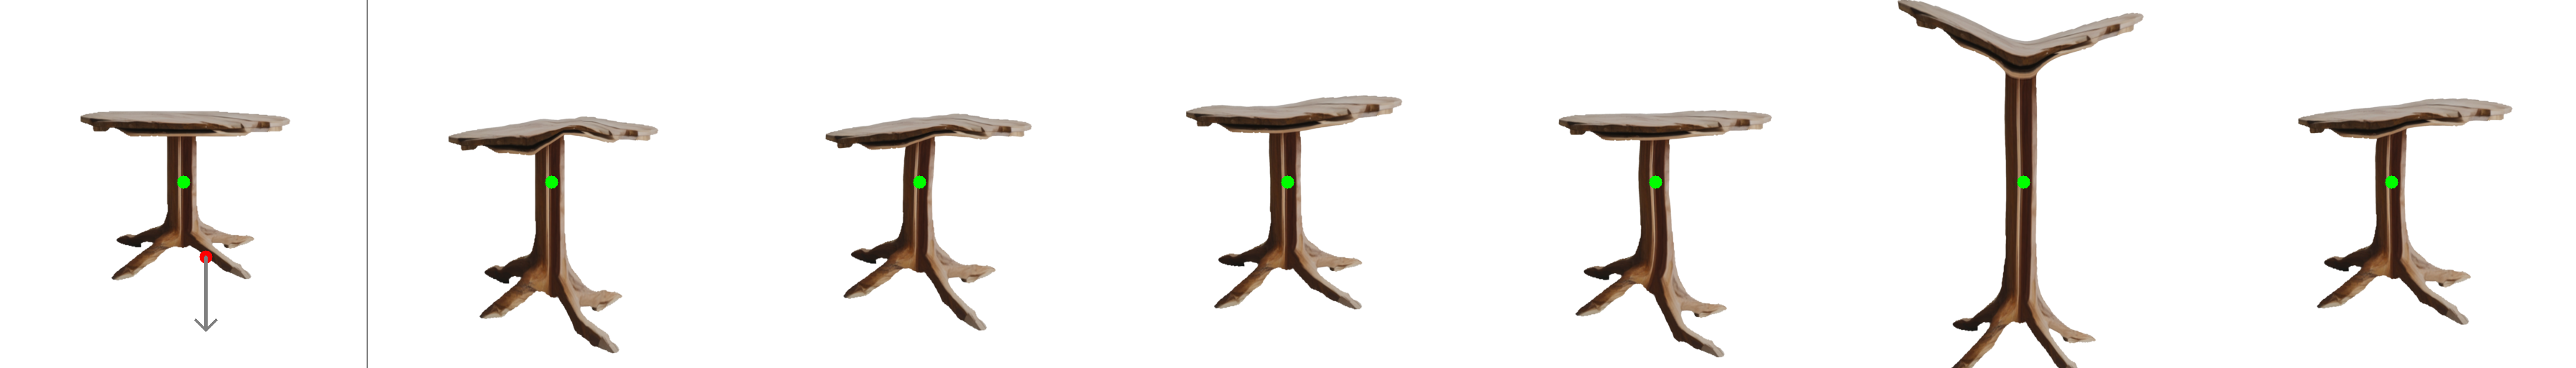}
